# Supplementary material for: Growth control of sessile microbubbles in PDMS devices
Source: arXiv:1510.01052 ancillary file (2015-12-02)
Supplement: Supplementary file 1 [file Supplementary.pdf]

**Growth control of sessile microbubbles in PDMS devices.**

# Supplementary Information: Estimation of permeabilities for $O_2$ through PDMS and water

Andreas Volk[a], Massimiliano Rossi[a], Christian J. Kähler[a], Sascha Hilgenfeldt[b], and Alvaro Marin[a]
[a] *Institute for Fluid Mechanics and Aerodynamics, Bundeswehr University Munich, 85577 Neubiberg, Germany and*
[b] *Department of Mechanical Science and Engineering, University of Illinois at Urbana Champaign, Urbana-Champaign, USA*

The aim of the following document is to demonstrate that the transport of air through PDMS is stronger than through liquid water at room conditions. In order to do so, we will calculate the relative permeability of oxygen through PDMS and an equivalent permeability through liquid water using its diffusivity and Henry's law. At the end of the document we will discuss the differences for the case of nitrogen and hydrogen.

Permeability data is normally found in the literature in the non-SI unit Barrer, which can be transformed using the following expression:

$$1 \text{ Barrer} = 3.348 \cdot 10^{-19} \frac{10^3 \text{mol} \cdot \text{m}}{\text{m}^2 \cdot \text{s} \cdot \text{Pa}} \tag{1}$$

We make use of the permeability data from Merkel et al. [1], which yields:

$$P^{\text{O}_2}_{\text{PDMS}} = 800 \text{ Barrer} = 2.67 \cdot 10^{-13} \frac{\text{mol}}{\text{m} \cdot \text{s} \cdot \text{Pa}} \tag{2}$$

We can define an equivalent permeability for oxygen in water as the following:

$$P^{\text{O}_2}_{\text{water}} = D^{\text{O}_2}_{\text{water}} K^{\text{O}_2}_{\text{water}} \tag{3}$$

Where $D^{\text{O}_2}_{\text{water}}$ is the diffusivity of oxygen in water, and $K^{\text{O}_2}_{\text{water}}$ is Henry's constant for oxygen in water. This expression can be easily obtained by calculating the volume of gas transferred through the liquid using Fick's type of transport and using Henry's law to express it in terms of partial pressures instead of concentrations.

Using the values taken from reference [2] and using the transformation in equation 1, we obtain:

$$P^{\text{O}_2}_{\text{water}} = 2 \cdot 10^{-5} \frac{\text{cm}^2}{\text{s}} 1.3 \cdot 10^{-3} \frac{\text{mol}}{\text{L} \cdot \text{atm}} = \tag{4}$$
$$= 2.6 \cdot 10^{-14} \frac{\text{mol}}{\text{m} \cdot \text{s} \cdot \text{Pa}}$$

The result is that oxygen is transferred through PDMS one order of magnitude more efficiently than through water at the same conditions. No significant differences are found for hydrogen and nitrogen. The values of the different constants are:

$$P^{\text{H}_2}_{\text{PDMS}} = 890 \text{ Barrer}$$
$$P^{\text{N}_2}_{\text{PDMS}} = 400 \text{ Barrer}$$
$$D^{\text{H}_2}_{\text{water}} = 4.5 \cdot 10^{-5} \frac{\text{cm}^2}{\text{s}}$$
$$D^{\text{N}_2}_{\text{water}} = 1.8 \cdot 10^{-5} \frac{\text{cm}^2}{\text{s}}$$
$$K^{\text{H}_2}_{\text{water}} = 7.8 \cdot 10^{-4} \frac{\text{mol}}{\text{L} \cdot \text{atm}}$$
$$K^{\text{N}_2}_{\text{water}} = 6.1 \cdot 10^{-4} \frac{\text{mol}}{\text{L} \cdot \text{atm}}$$

[1] T. Merkel, V. Bondar, K. Nagai, B. Freeman and I. Pinnau, *Journal of Polymer Science* Part B: Polymer Physics, 2000, 38, 415434.

[2] D. R. Lide, *CRC handbook of chemistry and physics*, CRC press, 2004

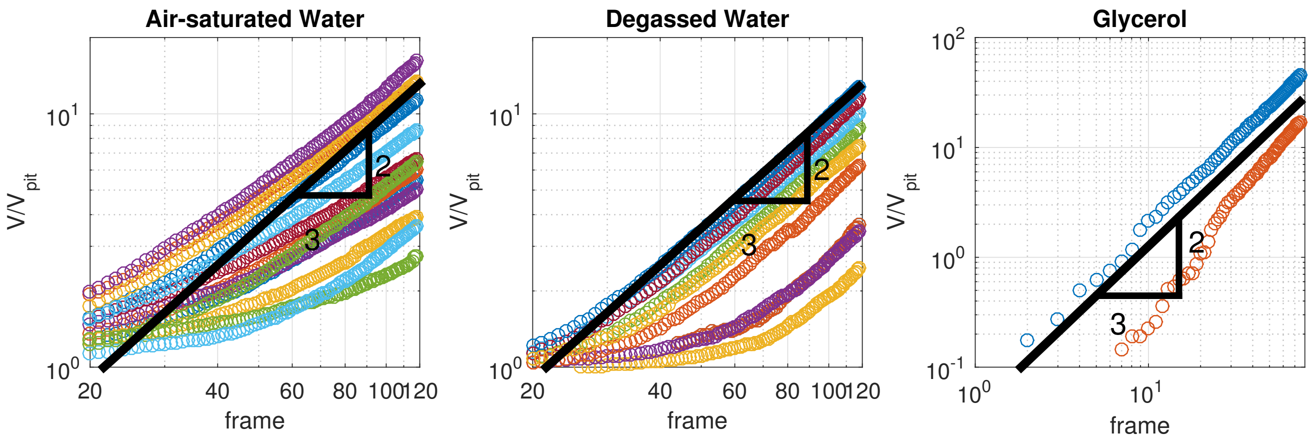


FIG. 1. This plot shows in detail the tendency towards the $V \sim t^{3/2}$ scaling of bubble volume with time for growing bubbles'. Note that such scaling would be expected for spherical bubbles growing in an homogeneous medium. The bubble's volume is normalized with the "pit" (blind channel) volume $V_{\rm pit}$. In all experiments the initial state is $V/V_{\rm pit} \approx 1$, and the growth tends to the mentioned scaling at larger time scales. Also note that the frame-rate-ratio is 0.2 frames per second.

Calculation of the area of PDMS exposed to the bubble: $A_s$
(See equation 7 in main text)

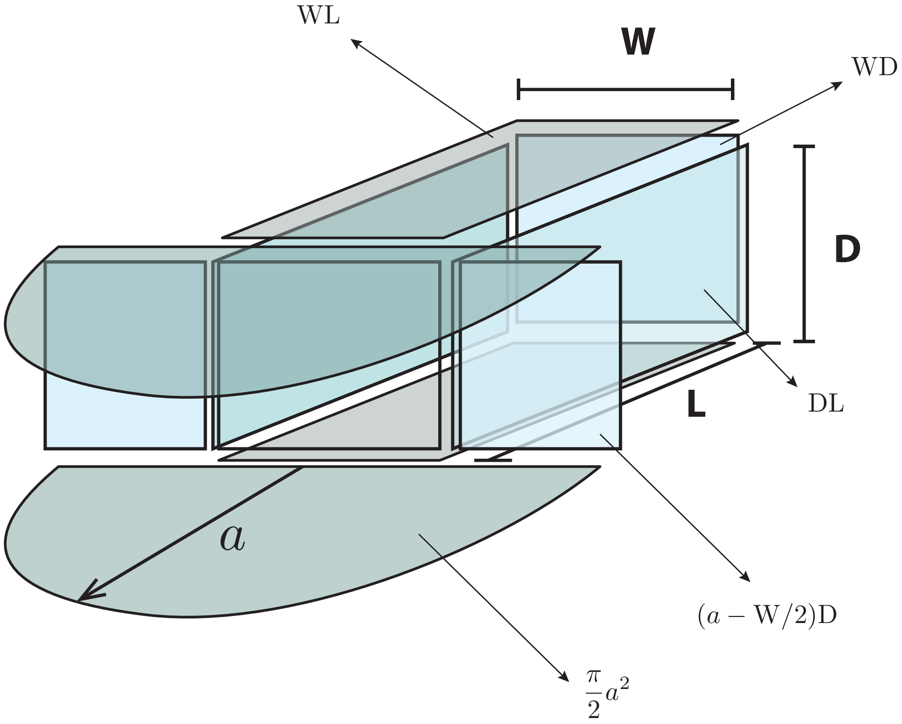


$$A_S = 2 \times \frac{\pi}{2}a^2 + 2 \times WL + 2 \times DL + WD + 2 \times (a - W/2)D$$
